# Supplementary material for: CORe: Capitalizing On Rewards in Bandit Exploration
Source: arXiv:2103.04387 source file (2021-03-07)
Supplement: Supplementary file 1 [file appendix_old.tex]

\section{Proof of \cref{theorem:gap-dependent-bound}}
\label{appendix:prove-bound}

\core is an instance of general randomized exploration algorithms in \citep{kveton2019garbage}. Thus the regret of \core can be analyzed using their Theorem 1. We first restate the Theorem here. 

For any arm $i$ and the number of its pulls $s\in[n]\cup\{0\}$, let $\hat{\mu} \sim p_t(\mathcal{H}_{i,s})$, where the distribution $p_t$ is a function of the reward history $\mathcal{H}_{i,s}$ of arm $i$ in each round and is defined by the specific randomized algorithm. Let
\begin{equation*}
    Q_{i,s}(\tau) = \condprob{\hat\mu\geq\tau}{\mathcal{H}_{i,s}}
\end{equation*}
be the tail probability that the estimated mean reward of arm $i$, $\hat\mu$, conditioned on history $\mathcal{H}_{i,s}$ is at least $\tau$ for some tunable parameter $\tau$. 

\begin{theorem}[\cite{kveton2019garbage}] 
\label{theorem:general_bound}
    For any tunable parameters $(\tau_i)_{i=2}^K\in\mathbb R^{K-1}$, the expected n-round regret of a randomized exploration algorithm can be bounded as $R(n)\leq \sum_{i=2}^K\Delta_i(a_i+b_i)$, where 
    \begin{align*}
        a_i &= \sum_{s=0}^{n-1} \E{\min\{1/Q_{1,s}(\tau_i)-1,n\}}, \\
        b_i &= \sum_{s=0}^{n-1} \prob{Q_{i,s}(\tau_i)>1/n}+1.
    \end{align*}
\end{theorem}
In \core, the mean reward estimate $\hat\mu$ of arm $i$ is given by line 15 in \cref{alg:core}, which is a specification of $p_t$ that depends on the sampled rewards from $\mathcal R_t$ in each round. Specifically, we set $\tau_i$ to be the average of the mean rewards of arm 1 and arm $i$, that is $\tau_i = \mu_i + \frac{\Delta_i}{2}$. Based on the above setting and the assumption of $16\alpha^2\log n\geq 1$, we can derive the gap-dependent regret bound in \cref{theorem:gap-dependent-bound} as follows.

First, after the initialization period, \cref{lemma:init-variance,lemma:bound_variance} states that with probability of at least $1-2/n$, sampling one i.i.d.\ reward from $\mathcal R_t$ satisfies two conditions: (1) has variance $\sigma^2(\mathcal R_t)\geq z\sigma^2/2$, and (2) follows a distribution that is $\max\{1,16\sigma^2\log n\}$-sub-Gaussian.
If either of these two conditions does not hold, the expected $n$-round regret incurred is at most $n\times 2/n=2$. % \todon{I am not sure if this claim is correct.}
Next we analyze the regret based on \cref{theorem:general_bound} when these two conditions hold. Note that from now on, for the second condition, we will only use the parameter $16\sigma^2\log n$ of the sub-Gaussianity for the worst case analysis, since $1$-sub-Gaussian will only gives us a regret bound with lower scaling with respect to $n$. Besides, The initial period will pull all arms sequentially for the first $\frac{2\log n}{z-1-\log z}$ rounds, which leads to at most $O(\log n)$ regret. We will show in the following analysis that when bounding $a_i$ and $b_i$ in \cref{theorem:general_bound}, this $O(\log n)$ regret from initialization is already covered by $O(\log^2 n)$ regret when the number of pulls of each arm is small than a threshold in the scale of $O(\log^2 n)$. 

\subsection{Upper Bound on $b_i$ in \cref{theorem:general_bound}} 
\label{sec:b_i}

Fix arm $i>1$ and choose $\tau_i=\mu_i+\Delta_i/2$. We have for $s>0$ that,
\begin{equation}
    Q_{i,s}(\tau_i) = \condprob{\frac{V_{i,s}+U_{i,s}}{s}\geq\mu_i+\frac{\Delta_i}{2}}{V_{i,s}}.
\end{equation}
We set $Q_{i,0}(\tau_i)=1$, due to the optimistic initialization that every arm is pulled at least once at the beginning. To simplify notation, we abbreviate $Q_{i,s}(\tau_i)$ as $Q_{i,s}$.

Fix the number of pulls $s$ of arm $i$, and let $m=512\alpha^2 \sigma^2\Delta_i^{-2}\log^2 n$. When $s\leq m$, we bound $\mathbb{P}(Q_{i,s}>1/n)$ trivially by 1. When $s\geq m$, we bound the term $b_i$ based on the event that $V_{i,s}$ is not much larger than its expectation, 
\begin{equation}
    E=\{V_{i,s}-\mu_is\leq\Delta_is/4\}.
\end{equation}
Then on event $E$,
\begin{align}
    Q_{i,s} &= \condprob{V_{i,s}+U_{i,s}-\mu_{i}s\geq \frac{\Delta_i}{2}s}{V_{i,s}} \\\nonumber
    &\leq\condprob{U_{i,s}\geq \frac{\Delta_i}{4}s}{V_{i,s}} \\\nonumber
    &\leq \exp\Big(-\frac{\Delta_i^2s}{512\alpha^2\sigma^2\log n}\Big) \leq n^{-1},
\end{align}
where the first inequality is by the definition of event $E$. The second is from Hoeffding's inequality on $U_{i,s}$, and the last is from $s>m$. On the other hand, event $\bar E$ is unlikely because
\begin{align}
\label{eq:b_unlike}
    \prob{\bar E} &= \prob{V_{i,s}-\mu_is\geq\Delta_is/4} \\\nonumber
    &\leq \exp\Big(-\frac{\Delta_i^2s}{32\sigma^2}\Big)\\\nonumber
    &\leq \exp\Big(-\frac{\Delta_i^2s}{512\alpha^2 \sigma^2\log n}\Big)\leq n^{-1},
\end{align} 
where the first inequality is by Hoeffding's inequality on Gaussian random variables, the second is by the assumption of $16\alpha^2\log n\geq 1$, and the last is based on the fact that $s>m$. % Note that the assumption of $16\alpha^2\log n\geq 1$ is easy to satisfy, e.g., we only need $\alpha \geq 1/4$ when $\log n>1$. % \todob{This needs to be an assumption in the theorem. Or clearly stated before it.}

Putting the above two inequalities together, we have
\begin{align}
    \prob{Q_{i,s}>1/n} = &\E{\prob{Q_{i,s}>1/n|V_{i,s}}\cdot\mathbbm 1\{E\}} \\ \nonumber
    &+
    \E{\prob{Q_{i,s}>1/n|V_{i,s}}\cdot\mathbbm 1\{\bar E\}} \\ \nonumber
    \leq & 0 + \prob{\bar E} \leq n^{-1}.
    \nonumber
\end{align}
Therefore, we can bound term $b_i$ in Theorem \ref{theorem:general_bound} as:
\begin{equation}
    b_i \leq 1 + \sum_{s=0}^{\lfloor m\rfloor}1 + \sum_{s=\lfloor m\rfloor+1}^{n-1}\frac{1}{n} \leq \frac{512\alpha^2 \sigma^2}{\Delta_i^2}\log^2 n + 3.
\end{equation}

\subsection{Upper Bound on $a_i$ in \cref{theorem:general_bound}}
\label{sec:a_i}

Fix arm $i>1$. As in \cref{sec:b_i}, we choose $\tau_i$ to be the average of the mean rewards of arm $1$ and arm $i$, $\tau_i=\mu_1-\Delta_i/2$. We have for $s>0$ that,
\begin{equation}
    Q_{1,s}(\tau_i) = \condprob{\frac{V_{1,s}+U_{1,s}}{s}\geq\mu_1-\frac{\Delta_i}{2}}{V_{1,s}}
\end{equation}

To simplify notation, we write $Q_{1,s}$ instead of $Q_{1,s}(\tau_i)$. Let $F_s=1/Q_{1,s}-1$. Fix the number of pulls $s$ of arm $1$, and let $m=1024\alpha^2\sigma^2\Delta_i^{-2}\log^2 n$.

\textbf{Case $s \leq m$:} notice that 
\begin{equation*}
    \E{F_s} \leq \E{1/Q_{1,s}} \leq \E{1/\condprob{U_{1,s} \geq \mu_1s-V_{1,s}}{V_{1,s}}}.
\end{equation*}
We can decompose $a_i$ by how much $V_{1,s}$ deviates from its mean $\mu_1s$. For any $\varepsilon>0$,
\begin{align}
\label{eq:a_i}
    &\E{\min\{F_s,n\}} \\ \nonumber
    &\leq \E{F_s\cdot\mathbbm 1\{\mu_1s-V_{1,s}\leq\varepsilon\}} + \E{n\cdot\mathbbm 1\{\mu_1s-V_{1,s}>\varepsilon\}} \\\nonumber
    &\leq \E{\frac{1}{\condprob{U_{1,s} \geq \mu_1s-V_{1,s}}{V_{1,s}}}\cdot\mathbbm 1\{\mu_1s-V_{1,s}\leq\varepsilon\}} \\\nonumber
    &\quad+ \E{n\cdot\mathbbm 1\{\mu_1s-V_{1,s}>\varepsilon\}} \\\nonumber
    &\leq \frac{1}{\prob{U_{1,s} \geq \varepsilon}} + n\cdot\prob{\mu_1 s - V_{1, s} > \varepsilon} %\E{n\cdot\mathbbm 1\{\mu_1s-V_{1,s}>\varepsilon\}},
\end{align}
where $\varepsilon$ quantifies how much $V_{1,s}$ deviates from $\mu_1s$ and the last step is from $\mu_1s - V_{1,s} \leq \varepsilon$.

Let us first focus on the second term in Eq~\eqref{eq:a_i}, which guides the choice of $\varepsilon$ for the rest of the proof. 
Specifically, let $\varepsilon^2=2s\sigma^2\log n$, we have:
\begin{equation}
    \prob{\mu_1s-V_{1,s}>\varepsilon} \leq\exp\bigg(-\frac{\varepsilon^2}{2s\sigma^2}\bigg) = n^{-1},
\end{equation}
which is the result of Hoeffding's inequality. %This gives $\E{n\cdot\mathbbm 1\{\mu_1s-V_{1,s}>\varepsilon\}} \leq 1$.

For the first term in Eq~\eqref{eq:a_i}, we need $\prob{U_{1,s}\geq \varepsilon}$ to be large enough to have an upper bound on $1/\prob{U_{1,s}\geq \varepsilon}$.

\begin{restatable}[Anti-concentration.]{lemma}{anticoncentration}
\label{lemma:anti-concentration}
 Let $X$ be a $\tilde{\sigma}^2$-sub-Gaussian random variable with $\E X=0$ and $\var X = \E{X^2}=\bar \sigma^2$. Then for any $0<w<y$, $\prob{|X|>w}>\frac{\bar \sigma^2-w^2-4\tilde{\sigma}^2\exp(-y^2/2\tilde{\sigma}^2)}{y^2}$. 
\end{restatable}

In Lemma \ref{lemma:anti-concentration}, $\bar\sigma^2$ is the exact variance of $X$ and $\tilde{\sigma}$ is the sub-Gaussian parameter. The proof can be found in \cref{appendix:lemmas}. 

Apply Lemma \ref{lemma:anti-concentration} by letting $X=U_{1,s}$, $w=\varepsilon$, $\bar\sigma^2 = \var{U_{1,s}} \geq \frac{s\alpha^2z\sigma^2}{2}$, and $\tilde\sigma^2=16s\alpha^2\sigma^2\log n$. We can bound $\prob{|U_{1,s}| \geq \varepsilon}$ as 
\begin{align}
\label{eq:anti-concentration}
    &\prob{U_{1,s} \geq \varepsilon} = \frac{1}{2}\prob{|U_{1,s}| \geq \varepsilon} \\\nonumber
    % \geq& \frac{s\alpha^2 \sigma_r^2 - \varepsilon^2 - 4s\alpha^2\sigma'^2 \exp(-y^2/2s\alpha^2\sigma'^2)}{2y^2} \\\nonumber
    \geq& \frac{s\alpha^2 z\sigma^2 - 4s\sigma^2\log n - 128s\alpha^2\sigma^2 \exp(\frac{-y^2}{32s\alpha^2\sigma^2\log n})\log n}{4y^2} \\\nonumber
    \geq& \frac{\alpha^2v-4-128\alpha^2\exp(-\frac{b}{32\alpha^2})}{4b} = C
\end{align}
by setting $z=v\log n$ and $y=\sqrt{bs\sigma^2\log n} > \varepsilon$ with $b\log n>2$, where $b,v$ are positive constants and $\alpha^2 v > 4+128\alpha^2\exp(-\frac{b}{32\alpha^2})$. % \todob{What does this mean? Note that you ignored the last term in this argument. That can be made exponentially small. But still.} We chain the inequalities above and get:
Therefore, we have 
\begin{equation}
    \E{\min\{F_s,n\}} \leq 1/C + 1,
\end{equation}
where $C$ is a constant given by Eq~\eqref{eq:anti-concentration}.

\textbf{Case $s > m$:} we bound $a_i$ based on the event that $V_{1,s}$ is not much smaller than its expectation, 
\begin{equation}
    E = \{\mu_1s-V_{1,s}\leq \Delta_is/4\}.
\end{equation}
On event $E$, we have 
\begin{align}
    Q_{1,s} &= \prob{\mu_1s-V_{1,s}-U_{1,s}\leq \frac{\Delta_is}{2}|V_{1,s}} \\\nonumber
    &\geq \prob{-U_{1,s}\leq \frac{\Delta_is}{4}} \\\nonumber
    &= 1 - \prob{U_{1,s}<-\frac{\Delta_is}{4}} \\\nonumber
    &\geq 1 - \exp\Bigg(-\frac{\Delta_i^2s}{512\alpha^2 \sigma^2\log n}\Bigg) > 1 - \frac{1}{n^2}, 
\end{align}
where the first inequality is based on event $E$, the second is based on the Hoeffding's inequality, and the last is based on $s>m$. From the definition of $F_s$, we have
\begin{equation}
    F_s = \frac{1}{Q_{1,s}}-1 \leq \frac{n^2}{n^2-1} - 1 = \frac{1}{n^2-1} \leq n^{-1}
\end{equation}
when $n\geq 2$. On the other hand, event $\bar E$ is unlikely because
\begin{align}
    \prob{\bar E} &= \prob{V_{1,s}-\mu_1s \leq-\Delta_is/4} \\\nonumber
    &\leq \exp\Big(-\frac{\Delta_i^2s}{32\sigma^2}\Big) \\\nonumber
    &\leq \exp\Big(-\frac{\Delta_i^2s}{512\alpha^2\sigma^2\log n}\Big)\leq n^{-2},
\end{align}
where the first inequality is by Hoeffding's inequality, the second is by the same assumption as in Eq~\eqref{eq:b_unlike} and the last is from $s>m$. Putting the above inequalities together and summarize the case when $s>m$, we have,
\begin{align}
    &\E{\min\{F_s,n\}} = \E{\E{\min\{F_s,n\}\big|V_{1,s}}\mathbbm 1\{E\}} \\\nonumber 
    &+ \E{\E{\min\{F_s,n\}\big|V_{1,s}}\mathbbm 1\{\bar E\}} \\\nonumber
    %  &\leq \mathbb E\big[\mathbb E[F_s\big|V_{1,s}]\mathbbm 1\{E\}\big] + \mathbb E\big[n\cdot \mathbbm 1\{\bar E\}\big|V_{1,s}\big] \\\nonumber
    &\leq n^{-1} \prob{E} + n\cdot\prob{\bar E} \leq 2n^{-1}
\end{align}
for any $n\geq 2$.
% \todob{What is $\E{n}$? The conditioning on $V_{1, s}$ is all wrong. It needs to be in the inner expectation.} 

Finally, we conclude the bound on $a_i$ for all $s$ as %\todob{Choose any style and stick to it. I do not write colons before math environments, because they are natural extensions of the text flow. You sometimes write them and sometimes not.}
\begin{align}
    a_i &\leq 1 + \sum_{s=1}^{\lfloor m\rfloor}\bigg(\frac{1}{C}+1\bigg) + \sum_{s=\lfloor m\rfloor+1}^{n-1}2n^{-1} \\\nonumber 
    &\leq \bigg(\frac{1}{C}+1\bigg)\frac{1024\alpha^2\sigma^2\log^2 n}{\Delta_i^{2}} + 3,
\end{align}
where $C$ is given by Eq~\eqref{eq:anti-concentration}.


\section{Technical Lemmas}
\label{appendix:lemmas}

% \begin{lemma}
% \label{lemma:init-variance}
%     If the number of rewards $q\geq\frac{2\log n}{z-1-\log z}$, the sample variance in the reward pool is at least $z\sigma^2\,,z\in(0,1)$ with probability of at least $1-\frac{1}{n}$. 
% \end{lemma}

\subsection{Proof of Lemma \ref{lemma:init-variance}}

Given a random variable $X\sim\mathcal N(\mu,\sigma^2)$, and a sample of it $(x_i)_{i=1}^q$ of size $q$. The sample variance is 
\begin{equation*}
    S^2 = \frac{1}{q-1}\sum_{i=1}^q (x_i-\bar x)^2,
\end{equation*}
where $\bar x = \frac{1}{q}\sum_{i=1}^q x_i$ is the mean of these $q$ observations. $S^2$ follows a scaled chi-squared distribution with ($q-1$) degrees of freedom,
\begin{equation}
    S^2\sim\frac{\sigma^2}{q-1}\cdot\chi^2_{q-1}. 
\end{equation}
The mean of $\chi^2_{q-1}$ is $q-1$. Let $0<z<1$ and $F(z(q-1);q-1)=\mathbb P(S^2<z\sigma^2)$ be the cumulative distribution function (CDF) of $\chi^2_{q-1}$. Based on Chernoff bounds on the lower tail of the CDF \citep{dasgupta2003elementary}, we have
\begin{equation*}
    F(z(q-1);q-1)\leq(ze^{1-z})^{(q-1)/2}. 
\end{equation*}
Let $(ze^{1-z})^{(q-1)/2} \leq 1/n$ and solve for $q$, we have $P(S^2<z\sigma^2)\leq 1/n$, when $q\geq \frac{2\log n}{z-1-\log z}$. However, the empirical variance of this sample is 
\begin{equation}
    \hat\sigma^2 = \frac{1}{q}\sum_{i=1}^q (x_i-\bar x)^2 = \frac{q-1}{q}S^2.
\end{equation}
Thus, $\hat\sigma^2 \geq S^2$ as long as $q\geq 2$. 

Finally, note that the sampled values in the reward pool $\mathcal R_t$ are from a mixture of Gaussian distributions with different means, rather than a single Gaussian. Denote the sample variance of $q$ sampled values from a mixture of Gaussian with the same variance $\sigma^2$ by $\tilde S^2$. \cref{lem:general chi-square upper bound} claims that $\prob{S^2\leq \varepsilon^2} \geq \prob{\tilde S^2\leq \varepsilon^2}$, which completes the proof. 


\subsection{Proof of Lemma \ref{lemma:bound_variance}}

The maximum number of rewards in the reward pool is $n$. Each reward $X_i$ can be viewed as a sample from $X_i\sim\mathcal N(\mu_i,\sigma^2)$, where $\mu_i$ is the mean reward of the pulled arm. Based on Hoeffding's inequality, we have 
\begin{equation}
    \prob{X_i-\mu_i\geq \sqrt{2\sigma^2\log(n/\delta)}} \leq \delta/n.
\end{equation}
% that $X_i$ deviates from the mean $\mu_i$ by more than $\sqrt{2\sigma^2\log(n/\delta)}$ with probability of at most $\delta/n$.
Then with union bound, we have for all $(X_i)_{i=1}^n$, the probability of any of them being away from the mean by more than $\sqrt{2\sigma^2\log(n/\delta)}$ is smaller than $\delta$. As $\mu_i\in[0,1]$, we have for any $X_i, i\in[n]$, $$-\sqrt{2\sigma^2\log(n/\delta)}\leq X_i\leq \sqrt{2\sigma^2\log(n/\delta)}+1$$ with probability of at least $\delta$. 
% \todob{It is not clear how we get from here to $\max \set{1, \dots}$ in the main claim. It seems that you use some relation between sub-Gaussianity and variance. If yes, state it clearly and cite.}
Finally, with Hoeffding's inequality, for any bounded random variable $X$, if $X_i\in[a,b]$ for all $i\in [n]$, then it is sub-Gaussian with parameter $\tilde\sigma=\frac{b-a}{2}$ \citep{wainwright_2019}. Therefore, the sub-Gaussian parameter $\tilde \sigma^2$ of sampling a reward from the reward pool is $(\frac{2\sqrt{2\sigma^2\log(n/\delta)}+1}{2})^2$. When $2\sqrt{2\sigma^2\log(n/\delta)}\leq 1$, $\tilde \sigma^2=1$; and when $2\sqrt{2\sigma^2\log(n/\delta)}>1$, $\tilde \sigma^2=8\sigma^2\log(n/\delta)$. Let $\delta=1/n$ completes the proof.  


\subsection{Other Lemmas}

\anticoncentration* 
\begin{proof}
Since the variance of $X$ is $\bar\sigma^2$, we have
\begin{align*}
    \bar\sigma^2&=\E{X^2}=\E{X^2\cdot\mathbbm 1\{|X|<w\}} +
    \E{X^2\cdot\mathbbm 1\{w\leq|X|<y\}}+\E{X^2\cdot\mathbbm 1\{y\leq|X|\}}
\end{align*} 
The first term on the right can be easily bounded by $E[X^2]=E[X^2\cdot\mathbbm 1\{|X|<w\}]\leq w^2$. For the third term, we have % \todob{I have a hard time parsing the integral. The first two steps are the same. What does $\int_{y^2}^\infty \mathbb P(X^2>t)dt$ mean? Is it $\int_{t = y^2}^\infty \mathbb P(X^2>t)dt$. Note that $X$ is random. Not $y$. So we need to integrate over $X$. What happened to $X^2$ next to the indicator?}
\begin{align*}
    \E{X^2\cdot\mathbbm 1\{y\leq|X|\}} &= \int_{y^2}^{\infty}X^2 \prob{X^2=x} dx \\\nonumber
    &= \int_{y^2}^\infty \prob{X^2>t} dt \\\nonumber
    &= \int_{y^2}^\infty \prob{|X|>\sqrt{t}}dt \\\nonumber
    *&\leq \int_{y^2}^\infty 2\cdot exp\bigg(-\frac{t}{2\tilde\sigma^2}\bigg)dt \\\nonumber
    &= 2\cdot(-2\tilde\sigma^2)exp\bigg(-\frac{t}{2\tilde\sigma^2}\bigg)\bigg|_{y^2}^\infty \\\nonumber
    &= 4\tilde\sigma^2exp\bigg(-\frac{y^2}{2\tilde\sigma^2}\bigg)
\end{align*}
where the inequality in step $*$ is from the Hoeffding's inequality given that $X$ is sub-Gaussian with parameter $\tilde\sigma$. Then from the decomposition of the variance of $X$, we can bound the second term as 
\begin{equation*}
    \E{X^2\cdot\mathbbm 1\{w\leq|X|<y\}}  \geq \bar\sigma^2 - w^2 - 4\tilde\sigma^2exp(-\frac{y^2}{2\tilde\sigma^2}).
\end{equation*}
Finally, for the second term,  
\begin{align*}
    \E{X^2\cdot\mathbbm 1\{w\leq|X|<y\}} &< y^2 \E{\mathbbm 1\{w\leq|X|<y\}} \\\nonumber
    &\leq y^2\prob{|X|>w} \\\nonumber
    &\leq \bar\sigma^2-w^2-4\tilde\sigma^2exp\bigg(-\frac{y^2}{2\tilde\sigma^2}\bigg),
\end{align*}
which provides the lower bound of $\prob{|X|>w}$.
\end{proof}

\begin{lemma}
\label{lem:general chi-square upper bound} Let $Z = (Z_i)_{i = 1}^d$ be a vector of independent standard normal variables. Let $A \in \mathbb{R}^{d \times d}$ be an arbitrary matrix and $X = A Z$. Then for any $\varepsilon > 0$ and vector $v \in \mathbb{R}^d$, we have that
\begin{align*}
  \prob{\normw{X}{2}^2 \leq \varepsilon^2}
  \geq \prob{\normw{X + v}{2}^2 \leq \varepsilon^2}\,.
\end{align*}
\end{lemma}
\begin{proof}
Since $Z \sim \mathcal{N}(\mathbf{0}, I_d)$, we have that $X \sim \mathcal{N}(\mathbf{0}, A A\T)$. Let $Y = X + v$. Then we also have that $Y \sim \mathcal{N}(v, A A\T)$. The important properties of $X$ and $Y$ are that their covariance matrices are the same.

Now note the following. The quantity $\prob{\normw{Y}{2}^2 \leq \varepsilon^2}$ is the density of $Y$ within distance $\varepsilon$ of $\mathbf{0}$. Since $Y$ is centered at $\mu$, its density contours are symmetric and ellipsoidal, and the $\varepsilon$ constraint is a ball, we have that $\prob{\normw{Y}{2}^2 \leq \varepsilon^2}$ is maximized when $\mu = \mathbf{0}$. In other words, for any $v$, we have that
\begin{align*}
  \prob{\normw{X}{2}^2 \leq \varepsilon^2}
  \geq \prob{\normw{Y}{2}^2 \leq \varepsilon^2}\,.
\end{align*}
This concludes the proof.
\end{proof}
